# Supplementary material for: Collective dynamics of trail-interacting particles
Source: arXiv:2512.03950 source file (2026-10-12)
Supplement: Supplementary file 1 [file Supplementary.pdf]

# Supplemental Material for: "Collective dynamics of trail-interacting particles"

## I. DERIVATION OF STOCHASTIC DENSITY FUNCTIONAL THEORY

Our microscopic model consists of $N$ particles distributed along $L/a$ lattice sites, where $L$ is the system size and $a$ the lattice constant. The state of each site is described by two occupancy numbers, a particle occupancy $\rho_i$ and a trail occupancy $\phi_i$. For brevity, we denote the vector $\boldsymbol{n}_i = (\rho_i, \phi_i)$. Within a time step $\Delta t$, two types of dynamics may take place: (i) hopping between neighboring sites with probability $P_{i\to i\pm 1} = 2\rho_i k_{tr}\Delta t / (1+\exp[H(\phi_{i\pm 1}) - H(\phi_i)])$ and (ii) deposition of a trail with probability $\rho_i k_d \Delta t$. Here, we have defined a typical translational rate $k_{tr}$ and a typical deposition rate $k_d$.

We coarse-grain the microscopic lattice model into continuum equations (stochastic density functional theory) using the path-integral method of Biroli and Lefevre [1, 2] (and see also [3, 4]). We write the probability of a trajectory as

$$P\left[\{\boldsymbol{n}_i(t_j)\}_{i,j}\right] = \prod_{i,j} \left\langle \delta\left(\boldsymbol{n}_i(t_{j+1}) - \boldsymbol{n}_i(t_j) - \boldsymbol{J}_i(t_j)\right)\right\rangle_{\boldsymbol{J}}, \tag{1}$$

where the average is over the possible fluxes $\{\boldsymbol{J}_i(t_j)\}_{i,j}$. We consider the possible fluxes between site $i$ and $i+1$. For example, if a particle moves to the right from $i$ to $i+1$, we have $\boldsymbol{J}_i = (-1, 0) = -\boldsymbol{J}_{i+1}$, while a deposition at site $i$ is given by $\boldsymbol{J}_i = (0, 1)$.

To construct a field theory, we introduce conjugate fluctuating variables $\hat{\boldsymbol{n}}_i(t_j) = (\hat{\rho}_i(t_j), \hat{\phi}_i(t_j))$, and write the Dirac delta function in Eq. (1) explicitly. This yields

$$P\left[\{\boldsymbol{n}_i(t_j)\}_{i,j}\right] = \mathcal{N} \int \prod_{i,j} \mathrm{d}\hat{\boldsymbol{n}}_i(t_j)\, \mathrm{e}^{i\hat{\boldsymbol{n}}_i(t_j)\cdot(\boldsymbol{n}_i(t_{j+1}) - \boldsymbol{n}_i(t_j))} \left\langle \mathrm{e}^{-i\hat{\boldsymbol{n}}_i(t_j)\cdot \boldsymbol{J}_i(t_j)}\right\rangle_{\boldsymbol{J}}, \tag{2}$$

where $\mathcal{N}$ is an irrelevant normalization prefactor. Note that $i$ is an index when written as a subscript and is the imaginary unit ortherwise.

Inserting the abovementioned probabilities and fluxes, the average is given by (the time dependence is omitted for brevity)

$$\begin{aligned}\left\langle \mathrm{e}^{-i\hat{\boldsymbol{n}}_i\cdot\boldsymbol{J}_i}\right\rangle_{\boldsymbol{J}} = 1 &+ k_d \rho_i \mathrm{d}t \left(\mathrm{e}^{-i\hat{\phi}_i} - 1\right) \\ &+ 2k_{tr}\mathrm{d}t \left[\frac{\rho_i}{1+\exp[H(\phi_{i+1}) - H(\phi_i)]}\left(\mathrm{e}^{i(\hat{\rho}_i - \hat{\rho}_{i+1})} - 1\right)\right. \\ &+ \left.\frac{\rho_{i+1}}{1+\exp[H(\phi_i) - H(\phi_{i+1})]}\left(\mathrm{e}^{i(-\hat{\rho}_i + \hat{\rho}_{i+1})} - 1\right)\right].\end{aligned} \tag{3}$$

The $k_{tr}$ term corresponds to translation and the $k_d$ term to deposition.

We exponentiate Eq. (3) for small d$t$ and find that

$$P\left[\left\{\boldsymbol{n}_i\left(t_j\right)\right\}\right]=\int\prod_{i,j}\mathrm{d}\hat{\boldsymbol{n}}_i\left(t_j\right)\exp\left(-S\left[\left\{\boldsymbol{n}_i\left(t_j\right),\hat{\boldsymbol{n}}_i\left(t_j\right)\right\}\right]\right) \tag{4}$$

with the discrete action

$$\begin{aligned}S=-\sum_{i,j}\Bigg[&i\hat{\rho}_i\left(t_j\right)\left(\rho_i\left(t_{j+1}\right)-\rho_i\left(t_j\right)\right)+\frac{2k_{tr}\rho_i\mathrm{d}t}{1+\exp\left[H\left(\phi_{i+1}\right)-H\left(\phi_i\right)\right]}\left(e^{i\left(\hat{\rho}_i-\hat{\rho}_{i+1}\right)}-1\right)\\&+\frac{2k_{tr}\rho_{i+1}\mathrm{d}t}{1+\exp\left[H\left(\phi_i\right)-H\left(\phi_{i+1}\right)\right]}\left(e^{i\left(-\hat{\rho}_i+\hat{\rho}_{i+1}\right)}-1\right)\\&+i\hat{\phi}_i\left(t_j\right)\left(\phi_i\left(t_{j+1}\right)-\phi_i\left(t_j\right)\right)+k_d\rho_i\mathrm{d}t\left(\mathrm{e}^{-i\hat{\phi}_i}-1\right)\Bigg].\end{aligned} \tag{5}$$

The last term is the characteristic function of the Poissonian process, describing chemical deposition.

We take the limit of continuous space and time and expand to second order in the lattice spacing $a$. In addition, we expand the characteristic function of the Poissionian process to second order in $\hat{\phi}$. This amounts to estimating the trail distribution by a normal distribution, appropariate after sufficient deposition, due to the central limit theorem (this can also be justified by scaling arguments for large system size, where higher powers of $\hat{\phi}$ become negligible). The following action is obtained:

$$\begin{aligned}S=-\int dtdx\Big[&i\hat{\rho}\dot{\rho}+i\hat{\phi}\dot{\phi}-i\hat{\phi}k_d\rho-\frac{1}{2}\rho k_d\hat{\phi}^2\\&+D\left(i\partial_x\rho\partial_x\hat{\rho}-\rho\left(\partial_x\hat{\rho}\right)^2\right)+iD\rho\partial_x\hat{\rho}\partial_xH\left(\phi\right)\Big],\end{aligned} \tag{6}$$

where we denote $D=k_{tr}a^2$ as the diffusion constant. In this continuum limit, the probability is given by the path integral

$$P\left[\boldsymbol{n}\left(t,x\right)\right]=\int\mathcal{D}\hat{\boldsymbol{n}}\exp\left(-S\left[\boldsymbol{n}(t,x),\hat{\boldsymbol{n}}\right]\right) \tag{7}$$

Next, we apply a Hubbard-Stratonovich transformation to the fluctuating fields,

$$\begin{aligned}P\left[\boldsymbol{n}\left(t,x\right)\right]=&\,\mathcal{N}\int\mathcal{D}\hat{\rho}\mathcal{D}\hat{\phi}\mathcal{D}\eta\mathcal{D}\xi\exp\left[\int dtdx\,i\hat{\rho}\left(\dot{\rho}-D\partial_x\left(\partial_x\rho+\rho\partial_xH\left(\phi\right)\right)+\partial_x\left(\sqrt{2D\rho}\,\eta\right)\right)\right]\\&\times\exp\left[\int dtdx\,i\hat{\phi}\left(\dot{\phi}-k_d\rho-\sqrt{k_d\rho}\,\xi\right)\right]\times\exp\left[-\int dtdx\frac{1}{2}\left(\eta^2+\xi^2\right)\right]\\=&\,\mathcal{N}\int\mathcal{D}\eta\mathcal{D}\xi\,\exp\left[-\int dtdx\frac{1}{2}\left(\eta^2+\xi^2\right)\right]\\&\times\delta\left[\left(\dot{\rho}-D\partial_x\left(\partial_x\rho+\rho\partial_xH\left(\phi\right)\right)+\partial_x\left(\sqrt{2D\rho}\,\eta\right)\right)\right]\times\delta\left[\dot{\phi}-k_d\rho-\sqrt{k_d\rho}\,\xi\right].\end{aligned} \tag{8}$$

This is equivalent to the equations

$$\dot{\rho} = D\partial_{xx}\rho + D\partial_x\left(\rho\partial_x H\left(\phi\right)\right) - \partial_x\left(\sqrt{2D\rho}\,\eta\right),$$
$$\dot{\phi} = k_d\rho + \sqrt{k_d\rho}\,\xi, \tag{9}$$

where $\eta$ and $\xi$ are normalized, Gaussian white noises. The generalization to higher spatial dimensions is straightforward.

## II. DENSITY AND TRAIL STATIC STRUCTURE FACTORS

### A. Structure factors of the density

Following the analysis of the linearized dynamics in the main text, we introduce $\delta\rho = \rho - \rho_0$ and $\delta\phi = \phi - kt$. Linearizing Eqs. (9) and rescaling as in the main text, yields (in dimensionless form)

$$\begin{cases} \partial_{tt}\delta\rho + q^2\partial_t\delta\rho + khq^2\delta\rho = \frac{\Xi}{\sqrt{N}}, \\ \Xi = \sqrt{2}iq\partial_t\eta - \sqrt{k}hq^2\xi. \end{cases} \tag{10}$$

The Green's function associated with Eq. (10) is given by [Eq. (4) in the main text]

$$G(\tau, q) = \frac{e^{-q^2\tau/2}}{\sqrt{\left(q^2/2\right)^2 - q^2kh}}\sinh\left(\tau\sqrt{\left(q^2/2\right)^2 - q^2kh}\right). \tag{11}$$

In turn, the solution for the density reads

$$\delta\rho(t, q) = \frac{1}{\sqrt{N}}\int_0^t \Xi(s, q)G(t-s, q)\,ds.$$

The structure factor is then given by

$$\begin{aligned} S_\rho(t, q) = \langle\delta\rho(t, q)\delta\rho(t, -q)\rangle &= \frac{1}{N}\left\langle\int_0^t ds\int_0^t ds'\Xi(s, q)\Xi(s', -q)\rangle G(t-s, q)G(t-s', -q)\right\rangle \\ &= \frac{q^2}{N}\left\langle\int_0^t ds\int_0^t ds'\left(2\partial_s\eta(s, q)\partial_{s'}\eta(s', -q) + kh^2q^2\xi(s, q)\xi(s'-q)\right)G(t-s, q)G(t-s', -q)\right\rangle \\ &= \frac{q^2}{N}\left\langle\int_0^t ds\int_0^t ds'\big[2\eta(s, q)\eta(s', -q)G'(t-s, q)G'(t-s', -q)\right. \\ &\qquad\qquad \left. + kh^2q^2\xi(s, q)\xi(s'-q)G(t-s, q)G(t-s', -q)\big]\right\rangle \end{aligned}$$

where we integrated by parts on $s$ and $s'$. We then distribute the averages of the realization of the noises and get $\langle\eta(s,q)\eta(s',-q)\rangle = \langle\xi(s,q)\xi(s',-q)\rangle = \delta(s-s')\delta(q-q)$. The $\delta(q-q)$ is equal to unity upon rescaling with $L$, but should not be forgotten if one redimensionizes the equations. Finally, as $G(\tau,-q) = G(\tau,q)$,

$$S_\rho(t,q) = \frac{q^2}{N}\int_0^t ds\,\left[2G'(s,q)^2 + kh^2q^2G^2(s,q)\right]$$

For clarity, we write it explicitly

$$\begin{aligned} NS_\rho(t,q) = &\left(1+\frac{h}{2}\right)\left\{1 - \frac{e^{-q^2t}}{q^2-4hk}\left[-4hk + q^2\cosh\left(qt\sqrt{q^2-4hk}\right)\right]\right\} \\ &+ \left(1-\frac{h}{2}\right)\frac{e^{-q^2t}}{\sqrt{q^2-4hk}}q\sinh\left(qt\sqrt{q^2-4hk}\right) \end{aligned} \tag{12}$$

For $h > 0$, the structure factor converges at long times ($t \gg 1$) to the steady-state (SS) structure factor given in the main text:

$$S_\rho(t,q) \underset{t\to\infty}{\approx} \frac{1}{N}\left(1+\frac{h}{2}\right) \tag{13}$$

### B. Structure factor of the trail

Similar to the density, one can derive linearized equations in terms of the Fourier-transform of the trail density

$$\begin{cases} \partial_{tt}\delta\phi + q^2\left(\partial_t\delta\phi + hk\delta\phi\right) = \frac{\Lambda}{\sqrt{N}}, \\ \Lambda = \sqrt{k}\left(\partial_t\xi + q^2\xi - i\sqrt{2k}\,q\,\eta\right). \end{cases} \tag{14}$$

Note the different noise term $\Lambda \neq \Xi$. Making use of the Green's function defined above, we obtain

$$\delta\phi(t,q) = \int_0^t G(t-s,q)\,\Lambda(s,q)\,ds,$$

so that

$$\begin{aligned} S_\phi(t,q) = \langle\delta\phi(t,q)\delta\phi(t,-q)\rangle &= \left\langle\int_0^t ds\int_0^t ds'\Lambda(s,q)\Lambda(s',-q)G(t-s,q)\,G(t-s',-q)\right\rangle \\ &= \frac{k}{N}\left\langle\int_0^t ds\int_0^t ds'\left[(\partial_s+q^2)\eta(s,q)(\partial_{s'}+q^2)\eta(s',-q)\right.\right. \\ &\qquad \left.\left. + 2kq^2\xi(s,q)\xi(s',-q)\right]G(t-s,q)\,G(t-s',-q)\right\rangle \end{aligned}$$

where we have removed cross-terms in $\eta$ and $\xi$ as $\langle \eta\xi \rangle = 0$. By integrating by parts and integrating over $s'$, we obtain

$$S_\phi(t,q) = \frac{k}{N}\int_0^t ds\,\left[(G'(s,q) + q^2 G(s,q))^2 + 2kq^2 G^2(s,q)\right]$$

. Explicitly, this is given by

$$\begin{aligned} N\,S_\phi(t,q) = &\frac{k(2+h)+q^2}{2h\,q^2} \\ &+ \frac{e^{-q^2 t}}{-2h\,q^2\,(q^2-4hk)}\Bigg\{\Big[4hk^2(-2-h) \\ &+ q^2\left[q^2 + k(2-3h)\right]\cosh\left(qt\sqrt{q^2-4hk}\right) \\ &+ q\sqrt{q^2-4hk}\,\left[q^2+k(2-h)\right]\sinh\left(qt\sqrt{q^2-4hk}\right)\Big]\Bigg\}. \end{aligned}$$

For $h > 0$, the steady-state structure factor reads [Eq. (5) in the main text]

$$S_\phi(t,q) \underset{t\to\infty}{\approx} \frac{k(2+h)+q^2}{2h\,N\,q^2}. \tag{15}$$

This shows that at length scales larger than $\sqrt{\frac{1}{k(2+h)}}$, the interface $\phi$ behaves as a Brownian motion $\delta\phi(x) = \sqrt{\frac{k(2+h)}{2h}}W(x)$ where $W(x)$ is the Wiener process. At short distances, the structure factor scales as $\sim \frac{1}{2h}$, indicating that the interface $\phi$ displays Poisson fluctuations of amplitude $\frac{1}{\sqrt{2h}}$.

### C. Case $h = 0$

The case $h = 0$ is singular and cannot be readily obtained from the steady state defined above. Indeed, for $h = 0$, the system does not reach a steady state and the time-dependent dynamics should be properly analyzed. Inserting $h = 0$ in Eq. (9), we find that the density is decoupled from the trail field, leading to the following solution of the linear, rescaled field

$$\begin{cases} \delta\rho(t,q) = -iq\sqrt{\frac{2}{N}}\int_0^t G(t-s,q)\,\eta(s,q)\,ds, \\ G(t,q) = e^{-q^2 t}, \\ S_\rho(t,q) = \frac{1}{N}\left(1 - e^{-q^2 t}\right). \end{cases} \tag{16}$$

The trail density is solved by

$$\partial_t \delta\phi \simeq k\delta\rho + \sqrt{\frac{k}{N}}\,\xi,$$

solved by

$$\delta\phi(t,q) = \int_0^t \left( k\delta\rho(s,q) + \sqrt{\frac{k}{N}}\,\xi(s,q) \right) ds.$$

The structure factor reads

$$\begin{aligned} S_\phi(t,q) &= \langle \delta\phi(t,q)\delta\phi(t,-q)\rangle \\ &= \int_0^t ds \int_0^t ds' \left\langle \left( k\delta\rho(s,q) + \sqrt{\frac{k}{N}}\,\xi(s,q) \right) \left( k\delta\rho(s',-q) + \sqrt{\frac{k}{N}}\,\xi(s',-q) \right) \right\rangle . \end{aligned} \tag{17}$$

There are three terms to calculate

1.

$$\begin{aligned} \langle \delta\rho(s,q)\delta\rho(s',-q)\rangle &= \frac{2q^2}{N} \int_0^s du \int_0^{s'} dv\, G(s-u,q)G(s'-v,-q)\langle \eta_q(u)\eta_{-q}(v)\rangle \\ &= \frac{2q^2}{N} \int_0^s du \int_0^{s'} dv\, G(s-u,q)G(s'-v,-q)\,\delta(u-v) \\ &= \frac{2q^2}{N} \int_0^{\min(s,s')} G(s-u,q)G(s'-u,-q)\,du \end{aligned}$$

2. $\langle \xi\delta\rho\rangle = 0$

3. $\left\langle \int_0^t ds \int_0^t ds' \langle \xi(s,q)\xi(s',-q)\rangle \right\rangle = t$

Finally

$$\begin{aligned} S_\phi(t,q) &= \frac{2k^2q^2}{N} \int_0^t ds \left\{ \int_0^s ds' \int_0^{s'} du + \int_s^t ds' \int_0^s du \right\} G(s-u,q)G(s'-u,-q) + \frac{kt}{N} \\ &= \frac{kt}{N}\left(1 + \frac{2k}{q^2}\right) + \frac{-3k^2}{q^4} + \frac{e^{-q^2t}(-1+4e^{-q^2t})}{q^4} \\ &\underset{t\gg 1}{\approx} \frac{kt}{N}\left(1 + \frac{2k}{q^2}\right) \end{aligned}$$

This means that upon rescaling by $\sqrt{t}$, the trail field $\delta\phi(x)/\sqrt{t}$ behaves for $q \ll \sqrt{2k}$ as a Brownian interface with effective diffusion coefficient of $k^2$.

## III. DYNAMIC STRUCTURE FACTORS

Upon Fourier transformation in time and space, the linearized dynamics (10) and (14) respectively read:

$$\begin{cases} \left[-\omega^2 + i\omega q^2 + khq^2\right] \delta\rho = -\frac{1}{\sqrt{N}} \left[\sqrt{2}q\omega\eta + \sqrt{k}hq^2\xi\right] \\ \left[-\omega^2 + i\omega q^2 + khq^2\right] \delta\phi = \sqrt{\frac{k}{N}} \left[(i\omega + q^2)\xi - i\sqrt{2k}q\eta\right] \end{cases}$$

We obtain

$$\begin{cases} \delta\rho(\omega, q) = \frac{i}{\sqrt{N}} \frac{\sqrt{2}q\omega\eta + \sqrt{k}hq^2\xi}{q^2\omega + i(\omega^2 - khq^2)} \\ \delta\phi(\omega, q) = \sqrt{\frac{k}{N}} \frac{\omega\xi - \sqrt{2k}q\eta - iq^2\xi}{\omega q^2 + i(\omega^2 - khq^2)} \end{cases}$$

We deduce the dynamic structure factor of the density and the trail:

$$\begin{cases} \mathcal{S}_\rho\left(\omega, q\right) = \langle|\delta\rho(\omega, q)|^2\rangle = \frac{1}{N} \frac{q^2(kh^2q^2 + 2\omega^2)}{q^4\omega^2 + (\omega^2 - hkq^2)^2} \\ S_\phi\left(\omega, q\right) = \langle|\delta\phi(\omega, q)|^2\rangle = \frac{k}{N} \frac{2kq^2 + q^4 + \omega^2}{(\omega^2 - khq^2)^2 + q^4\omega^2} \end{cases} \tag{18}$$

The $(\omega^2 - c^2q^2)^2$ term in the denominator is the signature of a wave mode propagating with the speed $c = \sqrt{hk}$. A comparison with numerical simulations is given in Fig 1 and confirms the contribution of this ballistic wave mode.

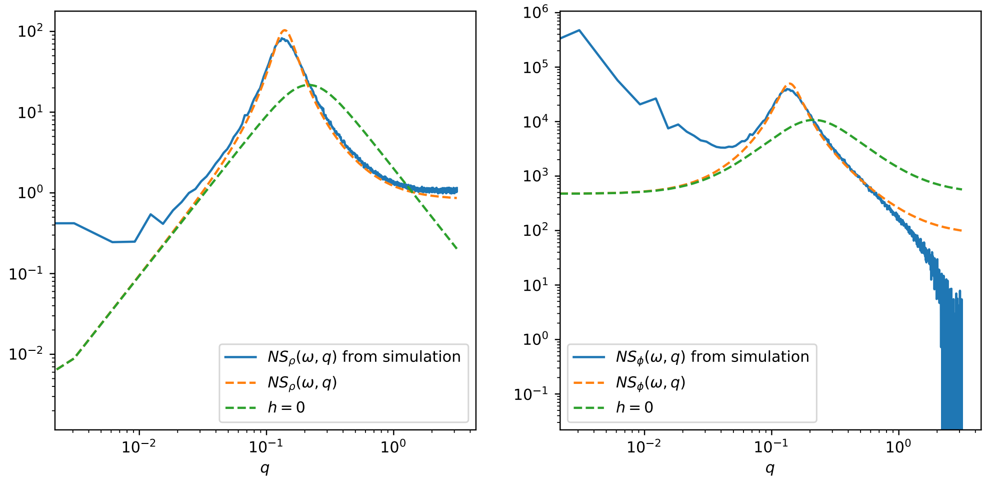


FIG. 1: Dynamical structure factor of the density (left) and of the trail (right). Solid lines are the results from simulations done with $h = 0.1, k = 1, \rho_0 = 1$ and $L = 2048$ sites, and measured at $\omega = 0.046$. Dotted lines represent theoretical predictions for $h = 0.1$ (orange) and for $h = 0$ (green).

## IV. DERIVATION OF MOVING-FRONT SOLUTION IN THE REPULSIVE CASE

The mean-field equations of our theory [Eq. (1) of the main text in the absence of noise] allow for traveling-front solutions in the repulsive case ($h > 0$). While they cannot be realized in our simulations due the periodic boundary conditions, we derive them analytically. First, we assume that the fields $\rho$ and $\phi$ depend on the moving coordinate $z = x - ct$, where $c$ is the velocity. This yields the following equations

$$\begin{aligned} -c\rho' &= \rho'' + h(\rho\phi')', \\ -c\phi' &= k\rho. \end{aligned} \tag{19}$$

Combining the two equations results in the ODE

$$\rho'' = -c\rho' \left(1 - \frac{2hk}{c^2}\rho\right). \tag{20}$$

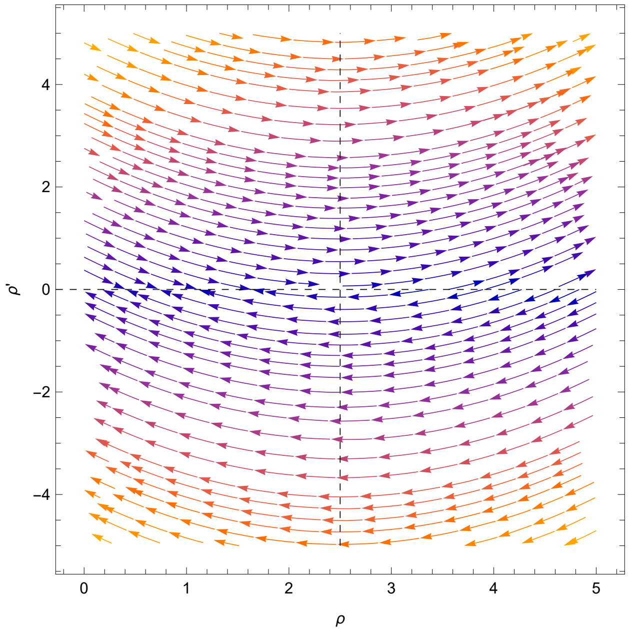


FIG. 2: Phase portrait of Eq. (20). A traveling front of decreasing density is represented by a contour that connects between $\rho_l$ and $\rho_r$, for which $\rho' = 0$ (intersections with the $x$ axis).

The phase portrait of this system is illustrated in Fig. 2. As long as $h > 0$, there is a density $\rho_* = c^2/2hk$, where $\rho''$ changes sign. This allows for a solution that connects $\rho_l > \rho_*$ at $z \to -\infty$ to $\rho_r < \rho_*$ at $z \to \infty$. The opposite trend (going from low to high density) does not hold. This means that it is possible to construct a steady traveling front but not a localized traveling packet within MF.

A solution to Eq. (20) can be found analytically, by inserting the ansatz

$$\rho = \rho_* \left(1 - \frac{\Delta\rho}{\rho_*} \tanh \frac{x}{\xi}\right) , \tag{21}$$

with $0 < \Delta\rho/\rho_* < 1$ and $\xi$ a coherence length. Knowing the average density $\langle\rho\rangle = \rho_0$, we require $\rho_* = \rho_0$. This provides the velocity

$$c = \sqrt{2hk\rho_0}. \tag{22}$$

Next, we calculate the derivatives and find

$$\begin{aligned} \rho' &= -\frac{\Delta\rho}{\xi} \left(1 - \tanh^2 \frac{x}{\xi}\right) , \\ \rho'' &= \frac{2\Delta\rho}{\xi^2} \tanh \frac{x}{\xi} \left(1 - \tanh^2 \frac{x}{\xi}\right) . \end{aligned} \tag{23}$$

Equating different powers of $\tanh x$ yields the coherence length in terms of the density difference $\xi = 2\rho_0/c\Delta\rho$. This provides a family of solutions

$$\rho = \rho_0 \left(1 - \frac{\Delta\rho}{\rho_0} \tanh \left[\frac{\Delta\rho}{2\rho_0} \sqrt{2hk\rho_0} \left(x - \sqrt{2hk\rho_0}t\right)\right]\right) , \tag{24}$$

for different $\Delta\rho$.

## V. MEAN FIELD SCALING SOLUTION FOR LOCALIZED INITIAL CONDITIONS

In this section, we determine the scaling solutions governing the dynamics for localized initial conditions in the vanishing-noise (mean-field) limit. We introduce the scaling ansatz

$$\begin{cases} \rho(t, x) = t^{-\alpha} f\left(\dfrac{x}{t^\alpha}\right) , \\ \phi(t, x) = t^{-\alpha+1} F\left(\dfrac{x}{t^\alpha}\right) , \end{cases}$$

and define the rescaled coordinate $u = x/t^\alpha$. Substituting this ansatz into Eq. (1), we obtain the coupled equations

$$\begin{cases} -\alpha t^{-\alpha-1}(fu)' = t^{-3\alpha} f''(u) + h\, t^{1-4\alpha}(fF')', \\ kf(u) = (1-\alpha)F(u) - \alpha u F'(u). \end{cases}$$

To capture the spatio-temporal evolution of $\rho$, we match the powers of $t$ on both sides of the first equation. Two distinct regimes emerge:

- **Diffusive regime:** For $\alpha = \frac{1}{2}$,

$$\begin{cases} -\dfrac{1}{2}(fu)' = f'' + ht^{1/2}(fF')', \\ kf(u) = \dfrac{1}{2}[F(u) - uF'(u)], \end{cases}$$

where the advection term is negligible for $t \ll 1/(kh)^2$, since $F \sim kf$. In this limit, the dynamics reduces to a diffusive behavior.

- **Superdiffusive regime:** For $\alpha = \frac{2}{3}$,

$$\begin{cases} -\dfrac{2}{3}(fu)' = t^{-1/3}f'' + h(fF')', \\ kf(u) = \dfrac{1}{3}[F(u) - 2uF'(u)], \end{cases}$$

where the diffusive term becomes negligible for $t \gg 1/(kh)^3$. In this regime, the system exhibits superdiffusive scaling.

These two scaling behaviors correspond to the regimes discussed in the main text. In what follows, we focus on the superdiffusive regime with $\alpha = 2/3$. Then the first equation yields

$$f \cdot (\frac{2}{3}u + hF') = C = 0,$$

where the last equality is due to the vanishing density at infinity. Then we have

$$\begin{cases} F(u) = \frac{1}{3h}\,(y_0^2 - u^2) \\ f(u) = \frac{1}{3hk}\,(u^2 + y_0^2/3)\,. \end{cases}$$

In order to find $y_0^2$, we know that $\phi$ is always positive, so $u$ must be in $[-y_0, y_0]$ (we suppose $y_0 > 0$). Furthermore, within MF, $\int_{-y_0}^{y_0} \phi(t,x)\,dx = Nkt$ and $\int_{-y_0}^{y_0} \rho(t,x)\,dx = N$. Both conditions gives $y_0 = \left(\frac{9Nkh}{4}\right)^{1/3}$. This allows us to obtain Eq. (9) of the main text. To confirm the prediction, we made fits of the parabolas for both fields. We set the notation for the parabola fitting function to be $P(x) = ax^2 + b$. We sum up the results in Fig. 3.

## VI. ATTRACTIVE CASE: SCALING OF $q_*$ WITH $k$

We plot in Fig. 4 the scaling of $q_*$ with $k$ in the strong interacting regime $|h| \gg 1$, as mentioned in the main text.

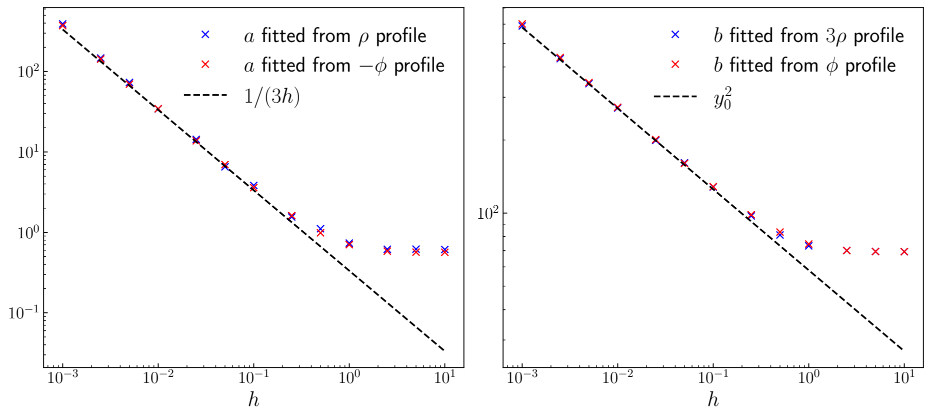


FIG. 3: Comparison of the theoretical predictions with the fitted parabola $P(x) = ax^2 + b$ parameters $a$ (left) and $b$ (right). Simulations are performed with $N = 1024$ and $k = 1$ and averaged over 100 realizations.

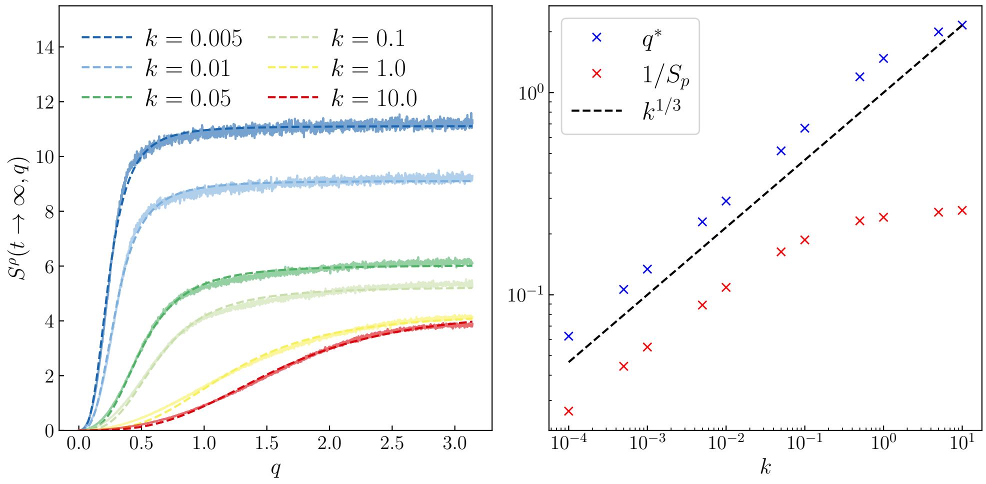


FIG. 4: The asymptotic value of the structure factor $S_p$ (left) and characteristic wavevector $q_*$ (right) as a function of $k$ for $h = -10$. The theoretical scaling is plotted in dashed black. Simulations are made for parameters values $L = 4096$, $k_{tr} = 1.$ and averaged $10^4$ times.

## VII. NUMERICAL SIMULATIONS

All numerical simulations were performed using the Gillespie algorithm implemented in `Julia`. All scripts required to reproduce the figures and analyses are available in a public repository:

`github.com/PaulPineauGit/Collective-dynamics-of-trail-interacting-particles`.

## VIII. SUPPLEMENTARY MOVIES

Videos of the dynamics are available at the GitHub repertory quoted above and `here`. There are done for the following values of parameters:

- $L = 256, h = -0.01, k_{tr} = 1, k = 1, \rho_0 = 1$
- $L = 256, h = -0.1, k_{tr} = 1, k = 1, \rho_0 = 1$
- $L = 256, h = 0.1, k_{tr} = 1, k = 1, \rho_0 = 1$


[1] A. Andreanov, G. Biroli, J.-P. Bouchaud, and A. Lefevre, Physical Review E **74**, 030101 (2006).

[2] A. Lefevre and G. Biroli, Journal of Statistical Mechanics: Theory and Experiment **2007**, P07024 (2007).

[3] S. Saha and T. Sadhu, SciPost Physics **17**, 033 (2024).

[4] R. Mukherjee, S. Saha, T. Sadhu, A. Dhar, and S. Sabhapandit, Physical Review E **111**, 024128 (2025).
